# Supplementary material for: Self-adjoint extension schemes and modern applications to quantum Hamiltonians
Source: arXiv:2201.10205 source file (2023-09-26)
Supplement: Supplementary file 2 [file appendix_Green.tex]

%%%%%%%%%%%%%%%%%%%%% appendix.tex %%%%%%%%%%%%%%%%%%%%%%%%%%%%%%%%%
%
% sample appendix
%
% Use this file as a template for your own input.
%
%%%%%%%%%%%%%%%%%%%%%%%% Springer-Verlag %%%%%%%%%%%%%%%%%%%%%%%%%%

% \appendix
\chapter{Green's methods}
\label{appendix_Green} % Always give a unique label
% use \chaptermark{}
% to alter or adjust the chapter heading in the running head

Use the template \emph{appendix.tex} together with the Springer document class SVMono (monograph-type books) or SVMult (edited books) to style appendix of your book in the Springer layout.

\section{Section}
